# Supplementary material for: Network Lasso: Clustering and Optimization in Large Graphs
Source: arXiv:1507.00280 source file (2015-07-01)
Supplement: Supplementary file 1 [file 090appendixA.tex]

To begin, we solve the consensus problem via ADMM to obtain $x^{\mathrm{cons}}$. When $\lambda \geq \lambda_\mathrm{critical}$, $x^{\mathrm{cons}}$ is the optimal solution at every node. Problem \eqref{GenCon} can be rewritten as
        \begin{equation*}
        \begin{array}{ll}
           \mbox{minimize}  &\sum\limits_{i \in \mathcal{V}}f_{i}(x_i) \\
           \mbox{subject to} &x_i = z_i, \quad i = 1,\ldots,m\\
           			      &x_i = z_j, \quad i = 1,\ldots,m, \quad j = N(i).
        \end{array}
        \end{equation*}
We introduce $z_i$, a copy of $x_i$, to insure equivalence to the original problem while also allowing for separability across the nodes. The Augmented Lagrangian is
        \begin{equation*}
        L_\rho(x,z,y) = \sum\limits_{i \in \mathcal{V}}f_i(x_i) + \sum\limits_{i \in \mathcal{V}}\underset{\substack{j \in N(i) \\ j = i}}{\sum} \left(y_{ij}^T(x_i - z_j) + (\rho/2)\|x_i - z_j\|_2^2 \right),
        \end{equation*}
and ADMM consists of the following iterations at each node:
	\begin{align*}
           &x_i^{k+1} = \underset{x_i}{\mathrm{argmin}} \left(f_i(x_i) +  \underset{\substack{j \in N(i) \\ j = i}}{\sum}(y_{ij}^T(x_i - z_j) + (\rho/2)\|x_i - z_j\|_2^2)\right)\\
           &z_i^{k+1} = \displaystyle\frac{\underset{\substack{j \in N(i) \\ j = i}}{\sum}x_j }{ \underset{\substack{j \in N(i) \\ j = i}}{\sum} 1}\\
           &y_i^{k+1} = y_i^{k} + \rho\underset{\substack{j \in N(i) \\ j = i}}{\sum}(x_i^{k+1} - z_j^{k+1}).
        \end{align*}
The $z$-update at node $i$ is just an average of the $x$'s neighboring $i$ \cite{BPCPE:11}. Unlike ADMM for the general problem, this update is node-separable, and there is no need to perform any operations at each edge. At every step $k$, node $i$ sends $x_i$, $z_i$, and $y_{i}$ to all of its neighbors. This process repeats and the resulting $x$, common across all nodes, is the consensus solution.

Given $x^{\mathrm{cons}}$, let $\mathcal{S}$ be a subset of the graph $\mathcal{G}$, and $\varepsilon$ be the edges from $\mathcal{S}$ to $\mathcal{S}^\mathsf{c}$, the complement of $\mathcal{S}$. For a given $\lambda$, If all other subsets are still optimal at $x_i = x^{\mathrm{cons}}, i = 1,\ldots,m$, subset $\mathcal{S}$ will ``break off'' if
  	\begin{equation*}
           0 \not\in \partial\left(\sum\limits_{i \in \mathcal{S}}f_{i}(x^{\mathrm{cons}}) + \lambda\sum\limits_{(i,j)\in \varepsilon} w_{ij} \|x^{\mathrm{cons}} - x_j\|_{2}\right),
        \end{equation*}
where $\partial$ denotes the subdifferential (of the objective in \eqref{original} evaluated at $x_j = x^{\mathrm{cons}}$). (FILL IN HERE). This condition holds for any
        \begin{equation*}
           \lambda \leq \displaystyle\frac{\left\|\sum\limits_{i \in \mathcal{S}}\nabla f_{i}(x^{\mathrm{cons}})\right\|}{\sum\limits_{(i,j)\in \varepsilon} w_{ij}}.
        \end{equation*}
Using this formula, $\lambda_{\mathrm{critical}}$ is simply the first subset of nodes which breaks off. This is equal to
        \begin{equation}  
           \lambda_{\mathrm{critical}} = \underset{\mathcal{S} }{\mathrm{argmax}} \left(\displaystyle\frac{\left\|\sum\limits_{i \in \mathcal{S}}\nabla f_{i}(x^{\mathrm{cons}})\right\|}{\sum\limits_{(i,j)\in \varepsilon} w_{ij}}  \right).
        \label{LambdaMax}
         \end{equation}
